# Supplementary material for: Experimental study of the initial growth of a localized turbulent patch in a stably stratified fluid
Source: arXiv:1603.06516 source file (2016-03-24)
Supplement: Supplementary file 1 [file appendix.tex]

\section{Appendix A}
\label{sec:appendix}

Possibly some discussion of local and conditional averaged quantities. The estimates in the paper using spatially averaged values, denoted by $\langle \cdot \rangle$. Careful look at the figure of buoyancy map shows that the spatially averaged quantities mask the behavior at small scales (of the order of the thickness of the interface) and underestimate the quantities such as $db/dz$. In order to quantify the real buoyancy gradient across the interface of a patch, we perform a so-called local analysis, in which quantities measured at each $x$ position and conditionally averaged shifting the profile around the local position of an interface, $z^*(x,t)$ (varying in space and time, $t$).  Shifting each profile, e.g. turbulent kinetic energy, $k(z-z^*,x,t)$ allows us to obtain a conditionally averaged (or phase averaged in respect to the distance from the interface) profiles, $\langle k(t) \rangle_{z^*}$. 

\begin{figure}
\caption{a) $\langle b(N,t=5.5) \rangle_x$, b) $b(x=0,N\,t=5.5)$, c) $\langle b \rangle_{z^*}$}
\end{figure} 

\begin{figure}
\caption{a) $\langle db/dz (N,t=5.5) \rangle_x$, b) $db/dz(x=0,N\,t=5.5)$, c) $\langle db/dz \rangle_{z^*}$}
\end{figure} 

We can try to get some better, local, gradient-based Richardson number, based on the local estimates. 

\begin{figure}
\caption{a) $Ri_1$, b) $Ri_2$, c) $Ri_3$}
\end{figure} 

\subsection{Interface conditional profiles}

\begin{figure}
\caption{ $\langle k(t) \rangle_{z^*}$}
\end{figure} 

\begin{figure}
\caption{ $\langle \omega^2(t) \rangle_{z^*}$}
\end{figure}
